# Supplementary material for: Ultrasensitive, universal single-ion nanodetector
Source: arXiv:2602.00406 source file (2026-11-24)
Supplement: Supplementary file 1 [file Supplement_CNT_ion_sensor.tex]

%% ****** Start of file aiptemplate.tex ****** %
%%
%%   This file is part of the files in the distribution of AIP substyles for REVTeX4.
%%   Version 4.1 of 9 October 2009.
%%
%
% This is a template for producing documents for use with 
% the REVTEX 4.1 document class and the AIP substyles.
% 
% Copy this file to another name and then work on that file.
% That way, you always have this original template file to use.

\documentclass[aip,graphicx]{revtex4-1}
%\documentclass[aip,reprint]{revtex4-1}
\usepackage{graphicx}
\usepackage{color}

\draft % marks overfull lines with a black rule on the right

\begin{document}

% Use the \preprint command to place your local institutional report number 
% on the title page in preprint mode.
% Multiple \preprint commands are allowed.
%\preprint{}

%Title of paper
\title{Supporting Information for: Ultrasensitive, universal single-ion nanodetector}

% repeat the \author .. \affiliation  etc. as needed
% \email, \thanks, \homepage, \altaffiliation all apply to the current author.
% Explanatory text should go in the []'s, 
% actual e-mail address or url should go in the {}'s for \email and \homepage.
% Please use the appropriate macro for the type of information

% \affiliation command applies to all authors since the last \affiliation command. 
% The \affiliation command should follow the other information.
\author{Namita Narendra}
\affiliation{Elmore Family School of Electrical and Computer Engineering, Purdue University, West Lafayette, Indiana 47907, United States}
\email{nnarendr@purdue.edu}

\author{Tillmann Kubis}
\affiliation{Elmore Family School of Electrical and Computer Engineering, Purdue University, West Lafayette, Indiana 47907, United States}
\email{tkubis@purdue.edu}


%\date{\today}

\maketitle

\setcounter{figure}{0}
\makeatletter
\renewcommand{\thefigure}{S\arabic{figure}}
\makeatother

\begin{figure}
  \centering
  \includegraphics[width=3.37in]{S1.png}
  \caption{Drain-source current densities of the CNT ion detector of Fig.~2 for different gate lengths - 6~nm (red), 8~nm (black), and 10~nm (blue) with (solid symbols) and without (open symbols) an ion in the nanodetector.
  }
  \label{figS1}
\end{figure}

\begin{figure}
  \centering
  \includegraphics[width=3.37in]{S2.png}
  \caption{Drain-source current densities of the larger diameter (19,0) CNT ion detector with a gate length of 10~nm with (red circles) and without (black squares) a positive ion in the CNT nanochannel under the gate. The ion induces a negative differential resistance for gate voltages above 0.3~V.
  }
  \label{figS2}
\end{figure}

\begin{figure}
  \centering
  \includegraphics[width=3.37in]{S3.png}
  \caption{Drain-source current density of the (11,0) p-type CNT ion detector with (red circles) and without (black squares) a negative ion in the CNT channel under the gate.
  }
  \label{figS3}
\end{figure}

\end{document}
